# Supplementary material for: Numerical Discretization Methods for the Extended Linear Quadratic Control Problem
Source: arXiv:2404.09316 source file (2024-04-14)
Supplement: Supplementary file 1 [file AppendixDistribution.tex]

\section*{Distribution of stochastic costs} \label{app:DistributionProofs}
